# Supplementary material for: Learning to Discretize: Solving 1D Scalar Conservation Laws via Deep Reinforcement Learning
Source: arXiv:1905.11079 source file (2020-10-05)
Supplement: Supplementary file 1 [file 06_appendix.tex]

\appendix

\section{Complementary Experiments}
\subsection{Comparison with supervised learning (SL) based methods}

We first note that most of the neural network based numerical PDE solvers cited in the introduction requires retraining when the initialization, terminal time, or the form of the PDE is changed; while the proposed RL solver is much less restricted as shown in our numerical experiments. This makes proper comparisons between existing NN-based solvers and our proposed solver very difficult. Therefore, to demonstrate the advantage of our proposed RL PDE solver, we would like to propose a new SL method that does not require retraining when the test setting (e.g. initialization, flux function, etc.) is different from the training. 

However, as far as we are concerned, it is challenging to design such SL methods without formulating the problem into an MDP. One may think that we can use WENO to generate the weights for the stencil at a particular grid point on a dense grid, and use the weights of WENO generated from the dense grid as the label to train a neural network in the coarse grid. But such setting has a fatal flaw in that the stencils computed in the dense grids are very different from those in the coarse grids, especially near singularities. Therefore, good weights on dense grids might perform very poorly on coarse grids. In other words, simple imitation of WENO on dense grids is not a good idea. One might also argue that instead of learning the weights of the stencils, we could instead generate the discrete operators, such as the spatial discretization of $\frac{\partial u_j}{\partial x}$, or the temporal discretization of $\frac{\partial u_j}{\partial t}$, the numerical fluxes $f_{j+\frac12}(u), f_{j-\frac12}(u)$, etc., on a dense grid, and then use them as labels to train a neural network in the supervised fashion on a coarse grid. However, the major problem with such design is that there is no guarantee that the learned discrete operators obey the conservation property of the equations, and thus they may also generalize very poorly.

% Here we compare our RL-based method with a SL-based method for learning to choose the stencil.
After formulating the problem into a MDP, there is indeed one way that we can use back-propagation (BP) instead of RL algorithms to optimize the policy network. 
Because all the computations on using the stencils to calculate the next-step approximations are differentiable, we can indeed use SL to train the weights. One possible way is to minimize the error (e.g. 2 norm) between the approximated and the true values, where the true value is pre-computed using a more accurate discretization on a fine mesh. The framework to train the SL network is described in Algorithm \ref{algo:sl}. Note that the framework to train the SL network is essentially the same as that of the proposed RL-WENO (Algorithm \ref{algo::RLprocedure}). The only difference is that we train the SL network using BP and the RL network using DDPG. 

 \begin{algorithm}
\small
	\SetKwProg{Fn}{Function}{:}{}
    \SetKwData{Input}{Input}{}
    \SetKwData{Output}{Output}{}
    \DontPrintSemicolon
    \Input : initial values $u^0_0, ... , u^0_J$, flux $f(u)$, $\Delta x$, $\Delta t$, evolve time $N$, left shift $r$, right shift $s$ and a neural network $\pi^{\theta}$ \\
    \Output : $\{U^n_j | ~j = 0, ..., J,~  n = 1, ..., N\}$ \\
    $U^0_j = u^0_j, ~j = 0, ..., J$ \\ 
    \For{Many iterations}
    {
    Construct initial states $s^0_j = g_s(U^0_{j-r-1}, ..., U^0_{j+s})$ for $j = 0, ..., J$ \\
    \For{$n = 1$ \KwTo $N$}
    {
      \For{$j = 0$ \KwTo $J$}
      {
    %   	Feed state $s^n_j$ to RL policy $\pi^{f}_{RL}$, get action $a^n_j = (\hat{f}^n_{j+\frac12}, \hat{f}^n_{j - \frac12})$ \\
        Compute the weights $(w_{j-\frac12}^{n,-2}, w_{j-\frac12}^{n,-1}, w_{j-\frac12}^{n,0}, w_{j-\frac12}^{n,1}, w_{j+\frac12}^{n,-2}, w_{j+\frac12}^{n,-1}, w_{j+\frac12}^{n,0}, w_{j+\frac12}^{n,1}) = \pi^{\theta}(s^n_j)$   \\
        Compute the fluxes $\hat{f}^n_{j - \frac12} = \sum_{i = -2}^1 w_{j-\frac12}^{n,i}\hat{f}^{n,i}_{j - \frac12}$, $\hat{f}_{j + \frac12} = \sum_{i = -2}^1 w_{j + \frac12}^i\hat{f}^{n,i}_{j + \frac12}$, where $\hat{f}^{n,i}_{j\pm\frac12}$ are the fluxes computed by WENO \\
        Compute $\frac{du_j(t)}{dt} 
      = -\frac{1}{\Delta x}(\hat{f}^n_{j + \frac12} - \hat{f}^n_{j - \frac12})$ \\
        Compute $U^{n}_j$ = $\pi^{t}(U^{n-1}_j, \frac{du_j(t)}{dt})$, e.g., the Euler scheme $U^{n}_j =  U^{n-1}_j + \Delta t \frac{du_j(t)}{dt}$ \\
      Compute the loss for $\theta$: $L^n_j(\theta) = || (U^n_{j-r-1}-u^n_{j-r-1},\cdots,U^n_{j+s}-u^n_{j+s}) - (U^n_{j-r-1}-u^n_{j-r-1},\cdots,U^n_{j+s}-u^n_{j+s}) ||_2^2$. \\
      Perform a gradient descent on $\theta$ w.r.t $L^n_j(\theta)$
      }
      
      Construct the next states $s^{n+1}_j = g_s(u^n_{j-r-1}, ..., u^n_{j+s})$ for $j = 0, ... ,J$ \\
    }	
    }
  \textbf{Return} the BP optimized policy $\pi^{\theta}$.
    \caption{Using BP instead of RL algorithm to train the policy}
    \label{algo:sl}
\end{algorithm}

However, we argue that the main drawback of using SL (BP) to optimize the stencils in such a way is that it cannot enforce long-term accuracy and thus cannot outperform the proposed RL-WENO. To support such claims, we have added experiments using SL to train the weights of the stencils, and the results are shown in table \ref{tab:RL-SL-weno-u2} and \ref{tab:RL-SL-weno-u4}. The SL policy is trained till it achieves very low loss (i.e., converges) in the training setting. However, as shown in the table, the SL-trained policy does not perform well overall. To improve longer time stability, one may argue that we could design the loss of SL to be the accumulated loss over multiple prediction steps, but in practice as the dynamics of our problem (computations for obtaining multiple step approximations) is highly non-linear, thus the gradient flow through multiple steps can be highly numerically unstable, making it difficult to obtain a decent result. 

\begin{table*}[htbp]
\tiny
\centering
\begin{tabular}{|c|c|c|c|c|c|c|c|c|c|}
\hline
\multirow{2}{*}{\diagbox{$\Delta t$}{$\Delta x$}} & \multicolumn{3}{c|}{0.02} & \multicolumn{3}{c|}{0.04} & \multicolumn{3}{c|}{0.05} \\ \cline{2-10} 
   & RL-WENO   &SL      & WENO         & RL-WENO    &SL     & WENO         & RL-WENO    &SL     & WENO         \\ \hline
0.002&  5.66 (1.59) & 7.86 (1.23) & 5.89 (1.74) &  8.76 (2.50) & 12.48 (0.78) & 9.09 (2.62) &  9.71 (2.42) & 12.14 (0.44) & 10.24 (2.84)  \\ \hline
0.003&  5.64 (1.54) & 7.77 (1.26) & 5.86 (1.67) &  8.73 (2.46) & 12.44 (0.78) & 9.06 (2.58) &  9.75 (2.41) & 12.13 (0.41) & 10.28 (2.81)  \\ \hline
0.004&  5.63 (1.55) & 7.72 (1.14) & 5.81 (1.66) &  8.72 (2.46) & 12.44 (0.64) & 9.05 (2.55) &  9.61 (2.42) & 12.14 (0.45) & 10.13 (2.84)  \\ \hline
0.005&  5.08 (1.46) & 7.14 (1.37) & 5.19 (1.58) &  8.29 (2.34) & 12.06 (0.86) & 8.58 (2.47) &  9.30 (2.26) & 11.86 (0.38) & 9.78 (2.69)  \\ \hline
0.006&  - & - & - &  8.71 (2.49) & 12.33 (0.73) & 9.02 (2.61) &  9.72 (2.38) & 12.14 (0.41) & 10.24 (2.80)  \\ \hline
0.007&  - & - & - &  8.56 (2.49) & 12.29 (0.83) & 8.84 (2.62) &  9.59 (2.41) & 12.06 (0.45) & 10.12 (2.80)  \\ \hline
0.008&  - & - & - &  8.68 (2.55) & 12.22 (0.70) & 8.93 (2.66) &  9.57 (2.49) & 12.08 (0.46) & 10.06 (2.92)  \\ \hline
 \end{tabular}

% % \vspace{0.05in}
 \caption{Comparison of relative errors ($\times 10^{-2}$) of RL-WENO, WENO, and SL-trained policy with standard deviations of the errors among 10 trials in the parenthesis. Temporal discretization: RK4; flux function: $\frac12 u^2$. RL-weno consistently outperforms WENO and SL-trained policy in all test cases. 
 } 
 \label{tab:RL-SL-weno-u2}
 \end{table*}
 
 \begin{table*}[htbp]
\tiny
\centering
\begin{tabular}{|c|c|c|c|c|c|c|c|c|c|}
\hline
\multirow{2}{*}{\diagbox{$\Delta t$}{$\Delta x$}} & \multicolumn{3}{c|}{0.02} & \multicolumn{3}{c|}{0.04} & \multicolumn{3}{c|}{0.05} \\ \cline{2-10} 
   & RL-WENO   &SL      & WENO         & RL-WENO    &SL     & WENO         & RL-WENO    &SL     & WENO         \\ \hline
0.002&  4.85 (1.15) & 5.84 (0.79) & 5.17 (1.26) &  7.77 (1.95) & 8.60 (1.12) & 8.05 (2.02) &  8.16 (1.93) & 8.42 (1.00) & 8.56 (2.19)  \\ \hline
0.003&  - & - & - &  7.79 (1.96) & 8.62 (1.12) & 8.06 (2.03) &  7.70 (1.96) & 8.42 (0.98) & 8.59 (2.18)  \\ \hline
0.004&  - & - & - &  7.72 (1.93) & 8.55 (1.15) & 7.98 (2.01) &  8.15 (1.95) & 8.41 (1.02) & 8.54 (2.20)  \\ \hline
0.005&  - & - & - &  - & - & - &  8.18 (1.94) & 8.40 (1.03) & 8.55 (2.15)  \\ \hline

 \end{tabular}

% % \vspace{0.05in}
 \caption{Comparison of relative errors ($\times 10^{-2}$) of RL-WENO, WENO, and SL-trained policy with standard deviations of the errors among 10 trials in the parenthesis. Temporal discretization: RK4; flux function: $\frac12 u^4$. RL-weno consistently outperforms WENO and SL-trained policy in all test cases.
 } 
 \label{tab:RL-SL-weno-u4}
 \end{table*}

\subsection{RL-weno's performance on smooth and singular regions $\frac{1}{16}u^4$}

\begin{figure*}[t]
    \centering
    \begin{tabular}{cc}
    % \includegraphics[width=0.45\textwidth]{img/conu2_fig.png} &
    % \includegraphics[width=0.45\textwidth]{img/disu2_fig.png} \\

    % (a) Smooth regions, $f(u) = \frac{1}{2}u^2$  & (b) Near singularities, $f(u) = \frac{1}{2}u^2$  \\
    
    \includegraphics[width=0.45\textwidth]{img/conu4_fig.png} &
    \includegraphics[width=0.45\textwidth]{img/disu4_fig.png} \\

     (c) Smooth regions, $f(u) = \frac{1}{16}u^4$  & (d) Near singularities, $f(u) = \frac{1}{16}u^4$  \\
  
    \end{tabular}
	\caption{These figures show the total number of grids whose error is under a specific value (i.e. the accumulated distribution function). The $x$-axis is the error in logarithmic (base 10) scale. (a) in smooth regions, (b) near singularities.}
	\label{fig:smooth-singular}
\end{figure*}

\subsection{Inference Time of RL-WENO and WENO}
In this subsection we report the inference time of RL-WENO and WENO. Although the computation complexity of the trained RL policy (a MLP) is higher than that of WENO, we could parallel and accelerate the computations using GPU. 

Our test is conducted in the following way: for each grid size $\Delta x$, we fix the initial condition as $u_0(x) = 1 + cos(6\pi x)$, the evolving time $T = 0.8$ and the flux function $f = u^2$. We then use RL-WENO and WENO to solve the problem 20 times, and report the average running time. For completeness, we also report the relative error of RL-WENO and WENO in each of these grid sizes in table \ref{tab::inference-error}. Note that the relative error is computed on average of several initial functions, and our RL-WENO policy is only trained on grid $(\Delta x, \Delta t) = (0.02, 0.004)$. 

For RL-WENO, we test it on both CPU and on GPU; For WENO, we test it purely on CPU, with a well-optimized version (e.g., good numpy vectorization in python), and a poor-implemented version (e.g., no vectorization, lots of loops). The CPU used for the tests is a custom Intel CORE i7, and the GPU is a custom  NVIDIA GTX 1080. The results are shown in table  \ref{tab::inference-time}.

\begin{table*}[htbp]
    \centering
    \begin{tabular}{c|c|c|c|c}
    $(\Delta x, \Delta t)$  & RL-WENO(CPU) & RL-WENO(GPU) & WENO-optimized  & WENO-poor \\ \hline
     (0.02, 0.004)   & 2.490 & 1.650 & \textbf{0.148} & 2.739 \\
     (0.01, 0.002)   & 7.720 &  1.700 & \textbf{0.349} & 10.778 \\ 
     (0.005, 0.001)  & 26.70 & 1.628  & \textbf{0.921}  & 44.23 \\
     (0.002, 0.0004)   & 110.92 & \textbf{1.611} & 1.961 & 277.88  \\
    \end{tabular}
    \caption{Average inference time (in seconds) for RL-WENO and WENO. Bold numbers are the smallest ones.}
    \label{tab::inference-time}
\end{table*}

\begin{table*}[htbp]
    \centering
    \begin{tabular}{c|c|c}
    $(\Delta x, \Delta t)$  & RL-WENO error & WENO error \\ \hline
     (0.02, 0.004)   & 3.73(0.40) & 4.08(0.23) \\
     (0.01, 0.002)   & 1.86(0.17) &  1.99(0.12)\\ 
     (0.005, 0.001)  & 1.00(0.05) & 0.93(0.01) \\
     (0.002, 0.0004)   & 0.48(0.03) & 0.39(0.02)  \\
    \end{tabular}
    \caption{Relative error of RL-WENO and WENO $(\times 10^{-2})$ on grid sizes tested in table \ref{tab::inference-time}. Note RL-WENO is only trained on grid $(\Delta x, \Delta t) = (0.02, 0.004)$}
    \label{tab::inference-error}
\end{table*}

From the table we can tell that as $\Delta x$ decreases, i.e., as the grid becomes denser, all methods, except for the RL-WENO (GPU), requires significant more time to finish the computation. The reason that the time cost of the GPU-version of RL-WENO does not grow is that on GPU, we can compute all approximations in the next step (i.e., to compute $(U^{t+1}_0, U^{t+1}_1, ..., U^{t+1}_J)$ given $(U^{t}_0, U^{t}_1, ..., U^{t}_J)$, which dominates the computation cost of the algorithm) together in parallel. Thus, the increase of grids does not affect much of the computation time. Therefore, for coarse grid, well-optimized WENO indeed has clear speed advantage over RL-WENO (even on GPU), but on a much denser grid, RL-WENO (GPU) can be faster than well-optimized WENO by leveraging the paralleling nature of the algorithm.  

\section{Review of Reinforcement Learning}

\subsection{Reinforcement Learning}
Reinforcement Learning (RL) is a general framework for solving sequential decision making problems. Recently, combined with deep neural networks, RL has achieved great success in various tasks such as playing video games from raw screen inputs~\citep{mnih2015human}, playing Go~\citep{silver2016mastering}, and robotics control \citep{schulman2017proximal}. The sequential decision making problem RL tackles is usually formulated as a Markov Decision Process (MDP), which comprises five elements: the state space $S$, the action space $A$, the reward $r: S \times A \rightarrow \mathcal{R}$, the transition probability of the environment $P: S \times A \times S \rightarrow [0, 1]$, and the discounting factor $\gamma$.  
The interactions between an RL agent and the environment forms a trajectory $\tau = (s_0, a_0, r_0, ..., s_T, a_T, r_T, ...)$. The return of $\tau$ is the discounted sum of all its future rewards:
$$G(\tau) = \sum_{t=0}^{\infty}\gamma^{t}r_{t}$$ Similarly, the return of a state-action pair $(s_t, a_t)$ is:
$$G(s_t, a_t) = \sum_{l=t}^{\infty}\gamma^{l-t}r_{l}$$
A policy $\pi$ in RL is a probability distribution on the action $A$ given a state $S$: $\pi: S \times A \rightarrow [0, 1]$. We say a trajectory $\tau$ is generated under policy $\pi$ if all the actions along the trajectory is chosen following $\pi$, i.e., $\tau \sim \pi$ means $a_t \sim \pi(\cdot | s_t)$ and $s_{t+1} \sim P(\cdot | s_t, a_t)$.   
Given a policy $\pi$, the value of a state $s$ is defined as the expected return of all the trajectories when the agent starts at $s$ and then follows $\pi$: 
$$V^{\pi}(s) = E_{\tau}[G(\tau) | \tau(s_0) = s, \tau \sim \pi]$$ 
Similarly, the value of a state-action pair is defined as the expected return of all trajectories when the agent starts at $s$, takes action $a$, and then follows $\pi$: $$Q^{\pi}(s,a) = E_{\tau}[G(\tau) | \tau(s_0) = s, \tau(a_0) = a, \tau \sim \pi]$$
As aforementioned in introduction, in most RL algorithms the policy $\pi$ is optimized with regards to the values $Q^{\pi}(s, a)$, thus  naturally guarantees the long-term accumulated rewards (in our setting, the long-term accuracy of the learned schemes).
Bellman Equation, one of the most important equations in RL, connects the value of a state and the value of its successor state:
\begin{equation*}
\begin{split}
     Q^{\pi}(s, a) &= r(s, a) + \gamma E_{s'\sim P(\cdot | s,a), a' \sim \pi(\cdot | s')}[Q^{\pi}(s', a')] \\
     V^{\pi}(s) &= E_{a \sim \pi(\cdot | s), s'\sim P(\cdot|s', a)}[r(s, a) + \gamma V^{\pi}(s')]
 \end{split}
\end{equation*}
The goal of RL is to find a policy $\pi$ to maximize the expected discounted sum of rewards starting from the initial state $s_0$, $J(\pi) = E_{s_0 \sim \rho}[V^{\pi}(s_0)]$, where $\rho$ is the initial state distribution. If we parameterize $\pi$ using $\theta$, then we can optimize it using the famous policy gradient theorem:
 \begin{equation*}\label{eq:rl-policygradient}
     \frac{dJ(\pi_\theta)}{d\theta} = E_{s \sim \rho^{\pi_\theta}, a \sim \pi_{\theta}}[\nabla_{\theta} \text{log}\pi_{\theta}(a | s) Q^{\pi_{\theta}}(s, a)]
 \end{equation*}
where $\rho^{\pi_\theta}$ is the state distribution deduced by the policy $\pi_\theta$.
 In this paper we focus on the case where the action space $A$ is continuous, and a lot of mature algorithms has been proposed for such a case, e.g., the Deep Deterministic Policy Gradient (DDPG) \citep{lillicrap2015continuous}, the Trust Region Policy Optimization algorithm \citep{schulman2015trust}, and etc.
